# Supplementary material for: Propensity weighting plus adjustment in proportional hazards model is not doubly robust
Source: arXiv:2310.16207 ancillary file (2025-05-30)
Supplement: Supplementary file 1 [file supplementary.pdf]

# Supplementary Materials: Propensity score weighting plus an adjusted proportional hazards model does not equal doubly robust away from the null

October 24, 2023

## S1 Proofs

### S1.1 Proof of misspecified PH model and correct propensity weighting of the score equations under the null

Let the true hazard for $T$ be $\lambda^\star(t|X, \boldsymbol{Z}; \boldsymbol{\omega})$, and working outcome model be

$$\lambda(t|X, \boldsymbol{Z}; \beta, \boldsymbol{\gamma}, \nu) = \lambda_0(t, \nu)\exp(\beta X + m(\boldsymbol{Z}; \boldsymbol{\gamma})), \tag{1}$$

as given in the main text.

Additionally, as in the main text, let $T_i$ be time until the event of interest for subject $i$, where $i = 1, \ldots, n$. We will occasionally omit the index where it is not needed. When there is (right) censoring, we will observe $\tilde{T}_i = \min\{T_i, C_i\}$ and $\Delta_i = I_{T_i \leq C_i}$ where $C_i$ is the censoring time. Let $X_i$ be the exposure of interest, which we assume is binary throughout. We need some additional notation for the proofs. Let $Y_i(t) = I_{\tilde{T}_i \geq t}$ and $N_i(t) = \Delta_i I_{\tilde{T}_i < t}$.

First assume our general working model, parametric or Cox semi-parametric, is in a randomized trial where $X \perp\!\!\!\perp \boldsymbol{Z}$, under the null of $T \perp\!\!\!\perp X|\boldsymbol{Z}$, and when censoring is both conditionally independent of survival time $T \perp\!\!\!\perp C|(X, \boldsymbol{Z})$ and of exposure given covariates $C \perp\!\!\!\perp X|\boldsymbol{Z}$ or $C \perp\!\!\!\perp \boldsymbol{Z}|X$. Then by Lemma 1 of DiRienzo and Lagakos [2001] $T \perp\!\!\!\perp C$, and by Kong and Slud [1997] we can write the (partial) score for $\beta$ of the working outcome model as:

$$n^{-1/2}U_\beta(\beta, \boldsymbol{\gamma}, \nu) = n^{-1/2}\sum_{i=1}^{n}\int\{X_i - \mu(t)\}\{dN_i(t) - p(t)Y_i(t)\lambda(t|X_i\boldsymbol{Z}_i; \beta, \boldsymbol{\gamma}^*, \nu^*)\} + o_p(1),$$

where $\boldsymbol{\gamma}^*$ and $\nu^*$ are the unique values that under standard regularity conditions the restricted maximum (partial) likelihood estimates $\hat{\boldsymbol{\gamma}}$ and $\hat{\nu}$ converge to as $n \to \infty$, the function $\mu(t) = \mathrm{E}\{X|Y(t) = 1\}$ and

$$p(t) = \frac{\mathrm{E}\{Y(t)\lambda^\star(t|X, \boldsymbol{Z}; \boldsymbol{\omega})\}}{\mathrm{E}\{Y(t)\lambda(t|X, \boldsymbol{Z}; \boldsymbol{\gamma}^*, \nu^*)\}}.$$

This follows from

$$\mathrm{E}\{X|Y(t) = 1, \boldsymbol{Z}\} = \mathrm{E}\{X|Y(t) = 1\}$$

due to the independence of $X$ and $\boldsymbol{Z}$ and the conditional independence of event time and censoring. Then, by theorem 2.1 of Kong and Slud [1997] $n^{-1/2}U_\beta(\beta, \hat{\gamma}, \hat{\nu}) \to_d N(0, \Sigma)$, and thus in a perfect randomized trial given the censoring conditions as outlined above, all proportional hazards models of the form we consider in the main text fit via (partial) maximum likelihood will be consistent under the null regardless of outcome model misspecification.

In a perfect randomized trial, the counterfactual event time is independent of randomization: $T(x) \perp\!\!\!\perp X$ for all $x$. Thus, the above proof also implies consistency of $\hat{\beta}$ under the null for the causal conditional log hazard ratio, and by the consistency of the Breslow estimator, the consistency of the regression standardization estimator for the causal survival difference at time $t$ when the average causal null holds $\mathrm{E}\{T(1)\} = \mathrm{E}\{T(0)\}$.

In order to move from the randomized trial setting to the observational study setting with IPT weighting, we must consider two different scenarios. As we state in the main text, if the working outcome model in (1) is correctly specified for censoring and confounding, then weighting by weights obtained from a misspecified propensity score model does not affect that this will be consistent in general. This can be seen by considering the component of the score corresponding to $\beta$ for the general proportional hazards model in (1)

$$\sum_{i=1}^{n} W(X_i, \boldsymbol{Z}_i; \hat{\boldsymbol{\alpha}}) \int \{X_i - \epsilon(\aleph, t)\} dM_i(t) + \int \left[ \sum_{i=1}^{n} W(X_i, \boldsymbol{Z}_i; \hat{\boldsymbol{\alpha}}) \{X_i - \epsilon(\boldsymbol{\aleph}, t)\} Y_i(t) \lambda^\star(t|X_i, \boldsymbol{Z}_i; \boldsymbol{\omega}) \right] dt \quad (2)$$

where $\boldsymbol{\aleph}$ is the vector of parameters $\{\beta, \boldsymbol{\gamma}, \nu\}$,

$$\epsilon(\boldsymbol{\aleph}, t) = \frac{\sum_j^n Y_j(t)\lambda(t|X_j, \boldsymbol{Z}_j; \beta, \boldsymbol{\gamma}, \nu) X_j}{\sum_j^n Y_j(t)\lambda(t|X_i, \boldsymbol{Z}_j; \beta, \boldsymbol{\gamma}, \nu)},$$

$M_i(t) = N_i(t) - \int Y_i(s)\lambda^\star(s|X_i, \boldsymbol{Z}_i, \boldsymbol{\omega}) ds \; \forall i \in \{1, \ldots, n\}$ is the local martingale in $t$ with respect to the filtration $(F_t) = \sigma\{N(s), Y(s^+), R : 0 < s \leq t\}$ representing the history of the process up to time $t$, and $W(X_i, \boldsymbol{Z}_i; \hat{\boldsymbol{\alpha}})$ is a bounded weight that is constant given the individual $i$.

Then, by Andersen et al. [2012] page 83, under the usual regularity conditions, the first part of this equation in (2) is asymptotically mean zero. The second term, by definition, will be zero when the true value of $\boldsymbol{\aleph}$ is substituted in, i.e., when the working outcome model and the true outcome model are the same, as this is simply the score which is set to zero by the weighted estimating equations in equation (8) of the main text. Thus if the working outcome model is correct then the estimate of $\boldsymbol{\aleph}$ is consistent for the truth and by consistency of the marginal survival estimator given the consistent parameters our estimator of the causal survival difference is also consistent.

We now consider the setting where the working outcome model is misspecified, but the propensity score is correctly specified for confounding. For this, we must impose the censoring assumptions we state in the main text: that there is no interaction between $X$ and $\boldsymbol{Z}$ in the hazard for the censoring. We will write that, as in the main text,

$$\lambda_C(t|X, \boldsymbol{Z}) = \alpha_0(t) + \alpha_1(t, X) + \alpha_2(t, \boldsymbol{Z})$$

such that

$$P(C > t|X, \boldsymbol{Z}) = \exp\left(-A_0(t) - A_1(t, X) - A_2(t, \boldsymbol{Z})\right),$$

and where $A_k$ is the cumulative of $\alpha_k$ and such that $A_k(t, 0) = 0$.

Again, the true model is $\lambda^\star(t|1, \boldsymbol{Z}; \boldsymbol{\omega})$ but we now enforce that $\lambda^\star(t|1, \boldsymbol{z}; \boldsymbol{\omega}) = \lambda^\star(t|0, \boldsymbol{z}; \boldsymbol{\omega})$, thus we are under the statistical null, which implies the causal null due to exchangeability given $\boldsymbol{Z}$.

Let us first consider the working outcome model to be a Cox model, specified as in the main text, but also let $\boldsymbol{O}_i^0 = 1$ and

$$\boldsymbol{O}_i^1 = \left\{ \begin{array}{c} X_i \\ m^{'}(\boldsymbol{Z}_i, \boldsymbol{\gamma}) \end{array} \right\},$$

where $m^{'}(\boldsymbol{Z}_l, \boldsymbol{\gamma})$ is the vector of partial derivatives with respect to $\gamma$.

Then, using the results of Struthers and Kalbfleisch [1986] and Lin and Wei [1989], the partial score equation in (6) of the main text can be written as

$$\int_0^t \left[ s_1(u) - \frac{s_1(u, \boldsymbol{\theta})}{s_0(u, \boldsymbol{\theta})} s_0(u) \right] du = 0 \quad (3)$$

and has a unique solution $\boldsymbol{\theta}^* = (\beta^*, \boldsymbol{\gamma}^*)$ where

$$s_j(u) = E[W(X_i, \boldsymbol{Z}_i; \boldsymbol{\alpha}^\star) Y_i(u) \boldsymbol{O}_i^j \lambda^\star(u|X_i, \boldsymbol{Z}_i; \omega)]$$

and

$$s_j(u, \boldsymbol{\theta}) = E[W(X_i, \boldsymbol{Z}_i; \boldsymbol{\alpha}^\star) Y_i(u) \boldsymbol{O}_i^j \exp\left(\beta X_i + m(\boldsymbol{Z}_i \boldsymbol{\gamma})\right)].$$

Here, we denote that the propensity score model is correct by using $\boldsymbol{\alpha}^\star$ in the weights, which is true value of the $\boldsymbol{\alpha}$ from the true propensity score model.

In this setting, we need to see that if our working model is not $\lambda^\star(u|X_i\boldsymbol{Z}_i;\omega)$ that under the censoring condition and using the correct propensity score and, under the null, $\lambda^\star(t|1,\boldsymbol{z};\boldsymbol{\omega}) = \lambda^\star(t|0,\boldsymbol{z};\boldsymbol{\omega})$, that $\beta^* = 0$ is the solution to the above equations.

We will use the shorthand for under the null of, $\lambda^\star(t|1,\boldsymbol{z};\boldsymbol{\omega}) = \lambda^\star(t|0,\boldsymbol{z};\boldsymbol{\omega})$, as $\lambda^\star(u|\boldsymbol{Z}_i;\omega)$, which excludes $X$. Under this model, we can take the expectations of the first row of the scores, with respect to $\beta$ as

$$
\begin{aligned}
s_0(u) &= E[W(X_i,\boldsymbol{Z}_i;\boldsymbol{\alpha}^\star)Y_i(u)\lambda^\star(u|\boldsymbol{Z}_i;\omega)] \\
&= E[E[W(X_i,\boldsymbol{Z}_i;\boldsymbol{\alpha}^\star)Y_i(u)\lambda^\star(u|\boldsymbol{Z}_i;\omega)|X,\boldsymbol{Z}]] \\
&= E\left[E\left[\frac{X}{g(\boldsymbol{Z};\boldsymbol{\alpha}^\star)}|\boldsymbol{Z}\right]\exp\left(-\Lambda^\star(u|\boldsymbol{Z},\omega)\right)\exp\left(-A_0(t)-A_1(t,1)-A_2(t,\boldsymbol{Z})\right)\lambda^\star(u|\boldsymbol{Z},\omega)\right] \\
&+ E\left[E\left[\frac{1-X}{1-g(\boldsymbol{Z};\boldsymbol{\alpha}^\star)}|\boldsymbol{Z}\right]\exp\left(-\Lambda^\star(u|\boldsymbol{Z},\omega)\right)\exp\left(-A_0(t)-A_2(t,\boldsymbol{Z})\right)\lambda^\star(u|\boldsymbol{Z},\omega)\right] \\
&= E\left[\exp\left(-\Lambda^\star(u|\boldsymbol{Z},\omega)\right)\exp\left(-A_0(t)-A_2(t,\boldsymbol{Z})\right)\lambda^\star(u|\boldsymbol{Z},\omega)\right]\left(1-\exp\left(-A_1(t,1)\right)\right)
\end{aligned}
$$

$$
\begin{aligned}
s_1(u) &= E[W(X_i,\boldsymbol{Z}_i;\boldsymbol{\alpha}^\star)Y_i(u)X_i\lambda^\star(u|\boldsymbol{Z}_i;\omega)] \\
&= E[E[W(X_i,\boldsymbol{Z}_i;\boldsymbol{\alpha}^\star)Y_i(u)X_i\lambda^\star(u|\boldsymbol{Z}_i;\omega)|X,\boldsymbol{Z}]] \\
&= E\left[E\left[\frac{X}{g(\boldsymbol{Z};\boldsymbol{\alpha}^\star)}|\boldsymbol{Z}\right]\exp\left(-\Lambda^\star(u|\boldsymbol{Z},\omega)\right)\exp\left(-A_0(t)-A_1(t,1)-A_2(t,\boldsymbol{Z})\right)\lambda^\star(u|\boldsymbol{Z},\omega)\right] \\
&= E\left[\exp\left(-\Lambda^\star(u|\boldsymbol{Z},\omega)\right)\exp\left(-A_0(t)-A_1(t,1)-A_2(t,\boldsymbol{Z})\right)\lambda^\star(u|\boldsymbol{Z},\omega)\right]\exp\left(-A_1(t)\right)
\end{aligned}
$$

Similarly, when $\beta^* = 0$, the first row of the score equations with respect to $\beta$ are

$$
\begin{aligned}
s_0(u,\beta^*) &= E[W(X_i,\boldsymbol{Z}_i;\boldsymbol{\alpha}^\star)Y_i(u)\exp\left(m(\boldsymbol{Z}_i\boldsymbol{\gamma}^*)\right)] \\
&= E\left[\exp\left(-\Lambda^\star(u|\boldsymbol{Z},\omega)\right)\exp\left(-A_0(t)-A_2(t,\boldsymbol{Z})\right)\exp\left(m(\boldsymbol{Z}_i\boldsymbol{\gamma}^*)\right)\right]\left(1-\exp\left(-A_1(t,1)\right)\right)
\end{aligned}
$$

$$
\begin{aligned}
s_1(u,\beta^*) &= E[W(X_i,\boldsymbol{Z}_i;\boldsymbol{\alpha}^\star)Y_i(u)\boldsymbol{O}_i\exp\left(m(\boldsymbol{Z}_i\boldsymbol{\gamma}^*)\right)] \\
&= E\left[\exp\left(-\Lambda^\star(u|\boldsymbol{Z},\omega)\right)\exp\left(-A_0(t)-A_2(t,\boldsymbol{Z})\right)\exp\left(m(\boldsymbol{Z}_i\boldsymbol{\gamma}^*)\right)\right]\exp\left(-A_1(t,1)\right)
\end{aligned}
$$

$$
\frac{s_1(u,\beta^*)}{s_0(u,\beta^*)}s_0(u) = E\left[\exp\left(-\Lambda^\star(u|\boldsymbol{Z},\omega)\right)\exp\left(-A_0(t)-A_2(t,\boldsymbol{Z})\right)\lambda^\star(u|\boldsymbol{Z},\omega)\right]\exp\left(-A_1(t,1) = s_1(u)\right.
$$

and thus the first row of (3) is 0 at $\beta^* = 0$, when $\lambda^\star(t|1,\boldsymbol{z};\boldsymbol{\omega}) = \lambda^\star(t|0,\boldsymbol{z};\boldsymbol{\omega})$, and thus $\beta^* = 0$ is the unique solution to the weighted Cox score, among the vector of unique solutions $\boldsymbol{\theta}^*$.

Now consider a generic proportional hazards model as given in equation 2.2 of Kong and Slud [1997] page 848 or, again, our equation (4) in the main text.

$$
\lambda(t|X,Z;\beta,\gamma,\nu) = \lambda_0(t,z,\boldsymbol{\gamma},\nu)\ \exp(\beta X) \tag{4}
$$

The form of the score remains the same; it just now corresponds to equation (8) of the main text, and thus we have a unique solution $\beta^*$ from the unique vector of solutions $\boldsymbol{\aleph}^*$ where the form is:

$$
\int_0^t \left[s_1(u,\boldsymbol{\aleph}) - \frac{s_1(u,\boldsymbol{\aleph}|\boldsymbol{O})}{s_0(u,\boldsymbol{\aleph}|\boldsymbol{O})}s_0(u)\right]du = 0. \tag{5}
$$

Here, the $s_j(u)$ will remain the same as above as the same true hazard remains the same. For ease of notation let $\aleph_\beta = (\boldsymbol{\gamma}, \nu)$, thus $\aleph$ less $\beta$. Additionally, let,

$$\boldsymbol{O}_Z^j = \left\{ \begin{array}{c} X^j \\ 1 \\ \vdots \\ 1 \end{array} \right\}$$

where $\boldsymbol{O}_Z^j$ is a vector with the same dimension as $\aleph$, and define

$$R_j(u, \boldsymbol{Z}, \boldsymbol{\gamma}, \nu) = \left\{ \begin{array}{c} 1 \\ \frac{\partial^j}{\partial^j \aleph_\beta} \log \lambda_0(u, \boldsymbol{Z}, \boldsymbol{\gamma}, \nu) \end{array} \right\}$$

and

$$\rho_j(u, \boldsymbol{Z}, \boldsymbol{\gamma}, \nu) = \left\{ \begin{array}{c} \exp{(\beta X)} \lambda_0(u, \boldsymbol{Z}, \boldsymbol{\gamma}, \nu) \\ \exp{(\beta X)} \frac{\partial^j}{\partial^j \aleph_\beta} \lambda_0(u, \boldsymbol{Z}, \boldsymbol{\gamma}, \nu) \end{array} \right\}.$$

Where again, both vectors are of the same dimension as $\aleph$. Then

$$s_j(u, \aleph) = E\left[W(X_i, \boldsymbol{Z}_i; \boldsymbol{\alpha}^\star) Y_i(u) \lambda^\star(u|\boldsymbol{Z}_i; \omega) t(\boldsymbol{O}_i^j) R_j(u, \boldsymbol{Z}, \boldsymbol{\gamma}, \nu)\right]$$

$$s_j(u, \aleph|\boldsymbol{Z}) = E\left[W(X_i, \boldsymbol{Z}_i; \boldsymbol{\alpha}^\star) Y_i(u) t(\boldsymbol{O}_i^j) \rho(u, z, \boldsymbol{\gamma}, \nu)\right]$$

Where $t(\cdot)$ is the transpose of a vector.

We then focus specifically on the score for $\beta$, when both $\lambda^\star(t|1, \boldsymbol{z}; \boldsymbol{\omega}) = \lambda^\star(t|0, \boldsymbol{z}; \boldsymbol{\omega})$ and $\beta^* = 0$

$$s_1(u, \beta) \quad = \quad E\left[W(X_i, \boldsymbol{Z}_i; \boldsymbol{\alpha}^\star) Y_i(u) \lambda^\star(u|\boldsymbol{Z}_i; \omega) X_i^j\right],$$

which is equal to the $\beta$ row of the original $s_1(u)$ above.

$$s_1(u, \beta|\boldsymbol{Z}) \quad = \quad E\left[W(X_i, \boldsymbol{Z}_i; \boldsymbol{\alpha}^\star) Y_i(u) X_i \lambda_0(u, \boldsymbol{Z}, \boldsymbol{\gamma}, \nu)\right]$$

$$s_0(u, \beta|\boldsymbol{Z}) \quad = \quad E\left[W(X_i, \boldsymbol{Z}_i; \boldsymbol{\alpha}^\star) Y_i(u) \lambda_0(u, \boldsymbol{Z}, \boldsymbol{\gamma}, \nu)\right]$$

And following the same steps as above, we are done. Thus $\beta^* = 0$ solves the first equation in the system in 5 when $\lambda^\star(t|1, \boldsymbol{z}; \boldsymbol{\omega}) = \lambda^\star(t|0, \boldsymbol{z}; \boldsymbol{\omega})$ and is thus the unique solution within the unique vector of solutions $\aleph^*$ from the weighed parametric general proportional hazards model as given in (4).

It is of note that this proof would follow, with only minor additional complexity, if the working outcome model were

$$\lambda(t|X, \boldsymbol{Z}; \beta, \gamma, \nu) = \lambda_0(t, \boldsymbol{Z}, \boldsymbol{\gamma}, \nu) \exp(\beta X + \beta_{xz} X g(\boldsymbol{Z}))$$

For some known function $g(\cdot)$. The important piece for the proof to apply is that X must remain proportional to the hazard. We would now set $\beta^* = \beta_{xz} = 0$, and again under the null $\lambda(t|1, \boldsymbol{Z}; \beta, \gamma, \nu) = \lambda(t|0, \boldsymbol{Z}; \beta, \gamma, \nu)$

## S2 Simulation study design and methods

**Completely independent censoring**. We assume the following distributions:

$$
\begin{aligned}
Z_1 &\sim \text{Normal}(0,1)\\
Z_2 &\sim \text{Normal}(2,1)\\
p_x &= \text{expit}(-1+0.3Z_1-0.3Z_2), X \sim \text{Bernoulli}(p_x)\\
\lambda_T &= \exp(\beta X+\log(2)Z_1+\log(6)Z_2-6), T \sim \text{Exponential}(\text{mean}=1/\lambda_T)\\
\gamma_C &= 0.35\,\text{median}(\lambda_T), C \sim \text{Exponential}(\text{mean}=1/\gamma_C),
\end{aligned}
$$

where $\text{expit}(x) = \exp(x)/\{1+\exp(x)\}$.
**Covariate-dependent censoring – Type A**. We assume the following distributions:

$$
\begin{aligned}
X &\sim \text{Bernoulli}(0.5),\\
Z_1 &\sim \text{Bernoulli}(0.3)\\
Z_2 &\sim \text{Bernoulli}(0.6)\\
\lambda_T &= \exp(\beta X+\log(2)Z_1-\log(4)Z_2)\\
T &\sim \text{Exponential}(\text{mean}=1/\lambda_T)\\
\gamma_{CX} &= \exp(-2+\log(10)X), \gamma_{CZ} = \exp(-2+\log(10)Z_2)\\
C &\sim \min\left\{\text{Exponential}(\text{mean}=1/\gamma_{CX}), \text{Exponential}(\text{mean}=1/\gamma_{CZ})\right\}.
\end{aligned}
$$

**Covariate-dependent censoring – Type B**. We assume the following distributions:

$$
\begin{aligned}
X &\sim \text{Bernoulli}(0.5)\\
Z_1 &\sim \text{Bernoulli}(0.3)\\
Z_2 &\sim \text{Bernoulli}(0.6),\\
\lambda_T &= \exp(\beta X+\log(2)Z_1-\log(4)Z_2)\\
T &\sim \text{Exponential}(\text{mean}=1/\lambda_T)\\
\gamma_C &= \exp(-2+\log(2)X+\log(2)Z_2+0.4Z_2X),\\
C &\sim \text{Exponential}(\text{mean}=1/\gamma_C).
\end{aligned}
$$

**Outcome-dependent censoring**. We assume the following distributions:

$$
\begin{aligned}
Z_1, Z_2, Z_3 &\sim \text{Normal}(0,1)\\
p_x &= \text{expit}(-1+0.3Z_1-0.3Z_2), X \sim \text{Bernoulli}(p_x)\\
\lambda_T &= \exp(\beta X+Z_1+Z_2), T \sim \text{Exponential}(\text{mean}=1/\lambda_T)\\
\gamma_C &= \exp(-2+\log(2.5)T-0.4X-2Z_3), C \sim \text{Exponential}(\text{mean}=1/\gamma_C).
\end{aligned}
$$

### S2.1 Analysis methods

**Completely independent censoring and outcome-dependent censoring**. We consider two models for the propensity score, both logistic regression, where the right model includes both $Z_1$ and $Z_2$ as linear predictors, and the wrong model includes only $Z_1$. In both cases, estimated propensity score weights are calculated as in the definition of $W(X, \boldsymbol{Z}; \hat{\boldsymbol{\alpha}})$.

We then fit Cox models where the linear predictor includes $X$ and $Z_1$ only (wrong model), with the right weights as case weights, where the linear predictor includes $X$, $Z_1$, and $Z_2$ (right model), with the wrong weights as case weights, and the wrong model with the wrong weights. These are all computed using the `coxph` function from the `survival` package in `R` with the propensity score weights given as the `weights` argument, and the Breslow method for ties.

We also fit proportional hazards Weibull models using the same outcome models as above, and with the same combinations of propensity score weights using the `flexsurvreg` function from the `flexsurv` package,

with the `dist = "weibullPH"` option. We also fit the flexible parametric model of Royston and Parmar using the same outcome models as above, and with the same combinations of right or wrong propensity score weights with the `flexsurvspline` function from the `flexsurv` package with the `scale = "hazard"` option.

From the above methods we report the conditional log hazard ratio for the $X$ variable and we estimate the regression standardized survival difference at time $t = 1$ using the formulas in Section **??**. We use the nonparametric bootstrap under the null settings to construct test statistics for assessing the type 1 error.

We fit the doubly robust procedure using a logistic model, as described in Blanche et al. [2023], for survival up to time $t = 1$ using the method described in Blanche et al. [2023] as implemented in the `logitIPCWATE` function of the `mets` package. For this we consider the cases where the outcome model contains linear terms for $X, Z_1$ and the propensity score model includes $Z_1, Z_2$ (wrong outcome, right weights), the outcome model contains $X, Z_1, Z_2$ and the propensity score model includes $Z_1$ (right outcome, wrong weights), and the wrong outcome, wrong weights combination. In this case the censoring distribution and censoring weights were estimated using the Kaplan-Meier method. We acknowledge that in this case the logistic model for the outcome is technically misspecified because the link function would not be logit, but we expect the bias induced by this to be quite small. The variance estimator implemented in the `mets` package is used for testing and assessing type 1 error.

For the doubly-robust method, we adapted the implementation described in Sjölander and Vansteelandt [2017] to estimate the survival difference and perform inference. We used parametric Weibull survival models as implemented in `survreg` for the outcome and the censoring distributions, and logistic regression for the propensity score model. As with the previous method, we consider the cases where the outcome model contains linear terms for $X, Z_1$ and the propensity score model includes $Z_1, Z_2$ (wrong outcome, right weights), the outcome model contains $X, Z_1, Z_2$ and the propensity score model includes $Z_1$ (right outcome, wrong weights), and the wrong outcome, wrong weights combination.

Finally, we fit the doubly robust pseudo observation method as described by Wang [2018] using the `cumincglm` function from the `eventglm` package with the option `link = "cloglog"` [Sachs and Gabriel, 2022]. Again, we consider the combinations where the outcome model is wrong, propensity score model is right, the outcome model is right, the propensity score model is wrong, and they are both wrong. We use bootstrap standard errors to construct test statistics for assessment of the type 1 error.

**Covariate-dependent censoring**. In this setting, we do not use propensity score weights because the exposure $X$ is completely randomized. For the Cox and parametric models, we consider the cases where the outcome model is correctly specified by including covariates $X, Z_1, Z_2$, and when it is misspecified by including covariates $X, Z_1$, and report the conditional log hazard ratios and the standardized survival differences.

For the logistic model, we use a Cox model to estimate the censoring distribution and consider the cases where the censoring model is correctly specified (by including $X, Z_2$ and their interaction) but the outcome model is misspecified, where the outcome model is correctly specified but the censoring model is misspecified (by including only $X$), and where both are misspecified. For the pseudo observation method, we account for covariate-dependent censoring by calculating the pseudo observations using the Kaplan-Meier estimator stratified by the categorical covariates. We consider cases where we stratify on $X, Z_2$ (censoring model right), and only on $X$ (censoring model wrong), and also where the outcome model is right or wrong.

# S3 Additional Simulation results

| setting | type | model | perc.bias.se |
|---|---|---|---|
| null_icens | right weights, wrong outcome | cox | 0.328 |
| null_icens | wrong weights, right outcome | cox | 0.047 |
| null_icens | wrong weights, wrong outcome | cox | 0.111 |
| null_icens | right weights, wrong outcome | dr | 0.010 |
| null_icens | wrong weights, right outcome | dr | 0.010 |
| null_icens | wrong weights, wrong outcome | dr | 0.007 |
| null_icens | right weights, wrong outcome | binreg | -0.002 |
| null_icens | wrong weights, right outcome | binreg | -0.012 |
| null_icens | wrong weights, wrong outcome | binreg | -0.001 |
| null_icens | right weights, wrong outcome | pseudo | 0.012 |
| null_icens | wrong weights, right outcome | pseudo | 0.007 |
| null_icens | wrong weights, wrong outcome | pseudo | 0.006 |
| nonnull_icens | right weights, wrong outcome | cox | 0.360 |
| nonnull_icens | wrong weights, right outcome | cox | 0.079 |
| nonnull_icens | wrong weights, wrong outcome | cox | 0.129 |
| nonnull_icens | right weights, wrong outcome | dr | 0.007 |
| nonnull_icens | wrong weights, right outcome | dr | 0.004 |
| nonnull_icens | wrong weights, wrong outcome | dr | -0.002 |
| nonnull_icens | right weights, wrong outcome | binreg | -0.008 |
| nonnull_icens | wrong weights, right outcome | binreg | -0.011 |
| nonnull_icens | wrong weights, wrong outcome | binreg | -0.008 |
| nonnull_icens | right weights, wrong outcome | pseudo | -0.001 |
| nonnull_icens | wrong weights, right outcome | pseudo | -0.002 |
| nonnull_icens | wrong weights, wrong outcome | pseudo | -0.006 |
| null_dcens | wrong outcome | cox | 0.010 |
| null_dcens | right outcome | cox | 0.008 |
| null_dcens | wrong outcome, right cens | dr | -0.024 |
| null_dcens | right outcome, wrong cens | dr | 0.006 |
| null_dcens | wrong both | dr | -0.022 |
| null_dcens | wrong outcome, right cens | binreg | -2.018 |
| null_dcens | right outcome, wrong cens | binreg | -2.032 |
| null_dcens | wrong both | binreg | -2.027 |
| null_dcens | wrong outcome, right cens | pseudo | -0.015 |
| null_dcens | right outcome, wrong cens | pseudo | -0.001 |
| null_dcens | wrong both | pseudo | -0.019 |
| nonnull_dcens | wrong outcome | cox | 0.010 |
| nonnull_dcens | right outcome | cox | 0.005 |
| nonnull_dcens | wrong outcome, right cens | dr | -0.025 |
| nonnull_dcens | right outcome, wrong cens | dr | -0.007 |
| nonnull_dcens | wrong both | dr | -0.017 |
| nonnull_dcens | wrong outcome, right cens | binreg | -2.042 |
| nonnull_dcens | right outcome, wrong cens | binreg | -2.059 |
| nonnull_dcens | wrong both | binreg | -2.061 |
| nonnull_dcens | wrong outcome, right cens | pseudo | -0.014 |
| nonnull_dcens | right outcome, wrong cens | pseudo | 0.000 |
| nonnull_dcens | wrong both | pseudo | -0.008 |
| null_tcens | right weights, wrong outcome | cox | 0.533 |
| null_tcens | wrong weights, right outcome | cox | 0.094 |
| null_tcens | wrong weights, wrong outcome | cox | 0.102 |
| null_tcens | right weights, wrong outcome | dr | -0.272 |
| null_tcens | wrong weights, right outcome | dr | -0.193 |
| null_tcens | wrong weights, wrong outcome | dr | -0.272 |
| null_tcens | right weights, wrong outcome | binreg | 0.032 |
| null_tcens | wrong weights, right outcome | binreg | 0.038 |
| null_tcens | wrong weights, wrong outcome | binreg | 0.043 |
| null_tcens | right weights, wrong outcome | pseudo | -0.025 |
| null_tcens | wrong weights, right outcome | pseudo | 0.017 |
| null_tcens | wrong weights, wrong outcome | pseudo | 0.026 |
| nonnull_tcens | right weights, wrong outcome | cox | 0.706 |
| nonnull_tcens | wrong weights, right outcome | cox | 0.229 |
| nonnull_tcens | wrong weights, wrong outcome | cox | 0.096 |
| nonnull_tcens | right weights, wrong outcome | dr | -0.157 |
| nonnull_tcens | wrong weights, right outcome | dr | -0.246 |
| nonnull_tcens | wrong weights, wrong outcome | dr | -0.039 |
| nonnull_tcens | right weights, wrong outcome | binreg | 0.033 |
| nonnull_tcens | wrong weights, right outcome | binreg | 0.052 |
| nonnull_tcens | wrong weights, wrong outcome | binreg | 0.024 |
| nonnull_tcens | right weights, wrong outcome | pseudo | -0.013 |
| nonnull_tcens | wrong weights, right outcome | pseudo | 0.013 |
| nonnull_tcens | wrong weights, wrong outcome | pseudo | 0.013 |



Table S1: Proprotion bias of the standard error estimators relative to the empirical

## S4 Code for the example analysis

```
library(survival)
library(stdReg)
library(eventglm)
library(mets)
library(data.table)
library(numDeriv)
library(boot)

#In IPW.fun and DR.fun: St0 should contain H0.t, H0.U, K0.t, and K0.U everywhere,
#not H.t, H.U, K.t, and K.U, but this doesn't matter since the latter are multiplied with
#(1-data[, A]) everywhere,  xcept in one place below where H0.t is used

afSurvival <- function(oformula = NULL, ofunc = "coxph", oarg = list(),
  cformula = NULL, cfunc = "coxph", carg = list(),
  eformula = NULL, earg = list(),
  method = "DR", times = NULL,
  rel.tol = .Machine$double.eps^0.1, jacobian.method = "simple",
  se.type = "none", data = NULL, weights = NULL, subset = NULL,
  R = 50, parallel = "no", cl = NULL, ncpus = NULL){

  if(!is.null(subset)) data <- data[subset, ]
  data <- na.omit(data)
  n <- nrow(data)
  if(is.null(weights)) weights <- rep(1, n)

  #---check that no left truncation, except if method == "ML"
  if((method == "IPW" | method == "DR") &
    length(as.character(oformula[[2]])) == 4)
    stop("Left truncation only allowed if method == ML", call. = FALSE)

  if(se.type == "boot"){

    bb <- boot(data = data, statistic = bootfun, R = R, parallel = parallel,
      cl = cl, ncpus = ncpus,
      oformula = oformula, ofunc = ofunc, oarg = oarg,
      cformula = cformula, cfunc = cfunc, carg = carg,
      eformula = eformula, earg = earg,
      method = method, times = times, rel.tol = rel.tol,
      ww = weights)

    est <- bb$t0
    se <-  apply(X = bb$t, MARGIN = 2, FUN = sd)
    out <- list(est.St = est[seq(1,3*length(times)-2,3)],
      se.St = se[seq(1,3*length(times)-2,3)],
      est.St0 = est[seq(2,3*length(times)-1,3)],
      se.St0 = se[seq(2,3*length(times)-1,3)],
      est.AF = est[seq(3,3*length(times),3)],
      se.AF = se[seq(3,3*length(times),3)])

  }

  if(se.type == "sandwich"){
```

```
    if((ofunc == "coxph" & (method == "ML" | method == "DR")) |
      (cfunc == "coxph" & (method == "IPW" | method == "DR")))
      stop("Sandwich estimator of variance not allowed for Cox models",
        call. = FALSE)

    fit <- afSurvival.fit(oformula = oformula, ofunc = ofunc, oarg = oarg,
      cformula = cformula, cfunc = cfunc, carg = carg,
      eformula = eformula, earg = earg,
      method = method, times = times,
      rel.tol = rel.tol, jacobian.method = jacobian.method,
      se.fit = TRUE, data = data, weights = weights)
    est <- fit$est
    se <- fit$se
    out <- list(est.St = est[seq(1,3*length(times)-2,3)],
      se.St = se[seq(1,3*length(times)-2,3)],
      est.St0 = est[seq(2,3*length(times)-1,3)],
      se.St0 = se[seq(2,3*length(times)-1,3)],
      est.AF = est[seq(3,3*length(times),3)],
      se.AF = se[seq(3,3*length(times),3)])

  }

  if(se.type == "none"){

    fit <- afSurvival.fit(oformula = oformula, ofunc = ofunc, oarg = oarg,
      cformula = cformula, cfunc = cfunc, carg = carg,
      eformula = eformula, earg = earg,
      method = method, times = times,
      rel.tol = rel.tol, jacobian.method = jacobian.method,
      se.fit = FALSE, data = data, weights = weights)
    est <- fit$est
    se <- fit$se
    out <- list(est.St = est[seq(1,3*length(times)-2,3)],
      est.St0 = est[seq(2,3*length(times)-1,3)],
      est.AF = est[seq(3,3*length(times),3)])

  }

  return(out)

}

bootfun <- function(data, indicies,
  oformula, ofunc, oarg,
  cformula, cfunc, carg,
  eformula, earg,
  method, times, rel.tol,
  ww){

  library(survival)

  weights <- ww
  n <- nrow(data)
```

```
  N <- sum(weights)
  #bootstrapping by weights: if(any(indicies != 1:n)) then the current call to
  #bootfun is not for the original data but for a bootstrap replicate. Then,
  #create a bootstrap replicate by assigning new weights according to the
  #distribution of the original weights. Otherwise, just pass on the
  #original weights.
  if(any(indicies != 1:n))
    weights <- rmultinom(n = 1, size = N, prob = weights/N)
  zeros <- (weights == 0)
  if(any(zeros)){
    weights <- weights[-which(zeros)]
    data <- data[-which(zeros), ]
  }
  out <- afSurvival.fit(oformula = oformula, ofunc = ofunc, oarg = oarg,
      cformula = cformula, cfunc = cfunc, carg = carg,
      eformula = eformula, earg = earg,
      method = method, times = times, rel.tol = rel.tol,
      se.fit = FALSE, data = data, weights = weights)
  return(out$est)

}

afSurvival.fit <- function(oformula, ofunc, oarg,
  cformula, cfunc, carg,
  eformula, earg,
  method, times, rel.tol, jacobian.method,
  se.fit, data, weights){

  #---SUBROUTINES---

  ML.fun <- function(theta){
    ofit.temp <- ofit
    if(!missing(theta)){
      if(ofunc == "survreg"){
        ofit.temp$coefficients <- theta[1:(nopar-1)]
        ofit.temp$scale <- exp(theta[nopar])
      }
      if(ofunc == "coxph") ofit.temp$coefficients <- theta
    }
    opred <- predict(object = ofit.temp, newdata = data, type = "lp")
    opred0 <- predict(object = ofit.temp, newdata = data0, type = "lp")
    if(ofunc == "survreg"){
      Stres <- 1-psurvreg(q = t, mean = opred, scale = ofit.temp$scale,
        distribution = ofit.temp$dist)
      St0res <- 1-psurvreg(q = t, mean = opred0, scale = ofit.temp$scale,
        distribution = ofit.temp$dist)
    }
    if(ofunc == "coxph"){
      #the standardized survival function could be estimated with survexp,
      #but that is MUCH slower
      sst <- survfit(formula = ofit.temp, se.fit = FALSE, censor = FALSE)
      Ststep <- stepfun(sst$time, c(1, sst$surv))
      Stres <- Ststep(t)^exp(opred)
      St0res <- Ststep(t)^exp(opred0)
```

```
  }
  out <- matrix(c(Stres, St0res), nrow = n, ncol = 2)
  if(!missing(theta))
    return(apply(X = out, MARGIN = 2, FUN = weighted.mean, w = weights,
      na.rm=TRUE))
  else return(out)
}

IPW.fun <- function(theta){
  cfit.temp <- cfit
  efit.temp <- efit
  if(!missing(theta)){
    if(cfunc == "survreg"){
      cfit.temp$coefficients <- theta[1:(ncpar-1)]
      cfit.temp$scale <- exp(theta[ncpar])
    }
    if(cfunc == "coxph") cfit.temp$coefficients <- theta[1:ncpar]
    efit.temp$coefficients <- theta[(ncpar+1):(ncpar+nepar)]
  }
  cpred <- predict(object = cfit.temp, newdata = data, type = "lp")
  if(cfunc == "survreg")
    Scres <- 1-psurvreg(q = t, mean = cpred, scale = cfit.temp$scale,
      distribution = cfit.temp$dist)
  if(cfunc == "coxph"){
    #the standardized survival function could be estimated with survexp,
    #but that is MUCH slower
    ssc <- survfit(formula = cfit.temp, se.fit = FALSE, censor = FALSE)
    Scstep <- stepfun(ssc$time, c(1, ssc$surv))
    Scres <- Scstep(t)^exp(cpred)
  }
  p <- predict(object = efit.temp, newdata = data, type = "response")
  Stres <- (data[, U] > t)/Scres
  St0res <- (1-data[, A])*(data[, U] > t)/((1-p)*Scres)
  out <- matrix(c(Stres, St0res), nrow = n, ncol = 2)
  if(!missing(theta))
    return(apply(X = out, MARGIN = 2, FUN = weighted.mean, w = weights,
      na.rm=TRUE))
  else return(out)
}

DR.fun <- function(theta){
  ofit.temp <- ofit
  cfit.temp <- cfit
  efit.temp <- efit
  if(!missing(theta)){
    if(ofunc == "survreg"){
      ofit.temp$coefficients <- theta[1:(nopar-1)]
      ofit.temp$scale <- exp(theta[nopar])
    }
    if(ofunc == "coxph") ofit.temp$coefficients <- theta[1:nopar]
    if(cfunc == "survreg"){
      cfit.temp$coefficients <- theta[(nopar+1):(nopar+ncpar-1)]
      cfit.temp$scale <- exp(theta[nopar+ncpar])
    }
```

```
  if(cfunc == "coxph")
    cfit.temp$coefficients <- theta[(nopar+1):(nopar+ncpar)]
  efit.temp$coefficients <- theta[(nopar+ncpar+1):(nopar+ncpar+nepar)]
}
opred <- predict(object = ofit.temp, newdata = data, type = "lp")
opred1 <- predict(object = ofit.temp, newdata = data1, type = "lp")
opred0 <- predict(object = ofit.temp, newdata = data0, type = "lp")
cpred <- predict(object = cfit.temp, newdata = data, type = "lp")
if(ofunc == "survreg")
  St.func <- function(r, opred)
    1-psurvreg(q = r, mean = opred, scale = ofit.temp$scale,
      distribution = ofit.temp$dist)
if(ofunc == "coxph"){
  #the standardized survival function could be estimated with survexp,
  #but that is MUCH slower
  sst <- survfit(formula = ofit.temp, se.fit = FALSE, censor = FALSE)
  Ststep <- stepfun(sst$time, c(1, sst$surv))
  St.func <- function(t, pred) Ststep(t)^exp(pred)
}
int.val <- vector(length = n)
if(cfunc  == "survreg"){
  Sc.func <- function(r, cpred)
    1-psurvreg(q = r, mean = cpred, scale = cfit.temp$scale,
      distribution = cfit.temp$dist)
  int.func <- function(r, opred, cpred){
    fc.r <- dsurvreg(x = r, mean = cpred, scale = cfit.temp$scale,
      distribution = cfit.temp$dist)
    Sc.r <- Sc.func(r, cpred)
    St.r <- St.func(r, opred)
    return(fc.r/(Sc.r^2*St.r))
  }
  int.val <- vector(length = n)
  for(i in seq(n)){
    int.try <- try(integrate(f = int.func, lower = 0,
      upper = min(data[i, U], t), opred = opred[i], cpred = cpred[i],
      rel.tol = rel.tol), silent = TRUE)
    if(class(int.try) == 'try-error') int.val[i] <- NA
    else int.val[i] <- int.try$value
  }
}
if(cfunc == "coxph"){
  #the standardized survival function could be estimated with survexp,
  #but that is MUCH slower
  ssc <- survfit(formula = cfit.temp, se.fit = FALSE, censor = FALSE)
  Scstep <- stepfun(ssc$time, c(1, ssc$surv))
  Sc.func <- function(t, pred) Scstep(t)^exp(pred)
  hc <- diff(-log(c(1, ssc$surv)))
  times.c <- ssc$time
  for(i in seq(n)){
    temp <- times.c < min(data[i, U], t)
    if(!any(temp)) int.val[i] <- 0
    else{
      upper <- max(which(times.c<min(data[i, U], t)))
      hc.i <- hc[1:upper]*exp(cpred[i])
```

```
        Sc.i <- Sc.func(times.c[1:upper], cpred[i])
        St.i <-  St.func(times.c[1:upper], opred[i])
        int.val[i] <- sum(hc.i/(Sc.i*St.i))
      }
    }
  }
  p <- predict(object = efit.temp, newdata = data, type = "response")
  H.t <- St.func(t, opred)
  H0.t <- St.func(t, opred0)
  H1.t <- St.func(t, opred1)
  K.t <- Sc.func(t, cpred)
  H.U <- St.func(data[, U], opred)
  K.U <- Sc.func(data[, U], cpred)
  int.t <- H.t*((1-data[, D])*(data[, U]<t)/(K.U*H.U)-int.val)
  int0.t <- (1-data[, A])/(1-p)*int.t
  int1.t <- (data[,A])/p * int.t
  ipw.term.t <- (data[, U] >= t)/K.t
  Stres <- ipw.term.t+int.t
  St0res <- (1-data[, A])/(1-p)*ipw.term.t-
    ((1-data[, A])-(1-p))/(1-p)*H0.t+int0.t
  St1res <- (data[, A])/(p)*ipw.term.t-
    ((data[, A])-(p))/(p)*H1.t+int1.t

  out <- matrix(c(St1res, St0res), nrow = n, ncol = 2)
  if(!missing(theta))
    return(apply(X = out, MARGIN = 2, FUN = weighted.mean, w = weights,
      na.rm=TRUE))
  else return(out)
}

#---PREPARATION---

n <- nrow(data)
N <- sum(weights)
A <- as.character(eformula[[2]])
data0 <- data1 <- data
data0[, A] <- 0
data1[, A] <- 1
est <- vector(length = length(3*times))
se <- vector(length = length(3*times))

if(method == "ML" | method == "DR"){
  D <- as.character(oformula[[2]])[length(as.character(oformula[[2]]))]
  oarg$formula <- oformula
  oarg$data <- data
  oarg$weights <- weights
  if(ofunc == "coxph") oarg$ties <- "breslow" #According to the manual,
  #the default is "efron", but it seems like the coxph function overrides
  #this and always uses "breslow" if the ties arise because of weights.
  #So for consistency, we set ties to "breslow".
  ofit <- do.call(ofunc, oarg)
  if(ofunc == "survreg") nopar <- length(ofit$coefficients)+1
  if(ofunc == "coxph") nopar <- length(ofit$coefficients)
  ofit <- do.call(ofunc, oarg)
```

```
  if(se.fit){
    if(ofunc == "coxph") ores <- residuals(object = ofit, type = "score")
    if(ofunc == "survreg"){
      rr <- residuals(object = ofit, type = "matrix")
      dldg <- rr[, "dg"]
      dgdx <- model.matrix(object = ofit)
      ores <- dldg*dgdx
      if(nrow(ofit$var) > length(ofit$coef)) ores <- cbind(ores, rr[, "ds"])
    }
    ovar <- -solve(ofit$var)/N
  }
}

if(method == "IPW" | method == "DR"){
  U <- as.character(cformula[[2]])[2]
  carg$formula <- cformula
  carg$data <- data
  carg$weights <- weights
  if(cfunc == "coxph") carg$ties <- "breslow" #According to the manual,
  #the default is "efron", but it seems like the coxph function overrides
  #this and always uses "breslow" if the ties arise because of weights.
  #So for consistency, we set ties to "breslow".
  cfit <- do.call(cfunc, carg)
  if(cfunc == "survreg") ncpar <- length(cfit$coefficients)+1
  if(cfunc == "coxph") ncpar <- length(cfit$coefficients)
  earg$formula <- eformula
  earg$data <- data
  earg$weights <- weights
  earg$family <- "binomial"
  efit <- do.call("glm", earg)
  nepar <- length(efit$coefficients)
  if(se.fit){
    if(cfunc == "coxph") cres <- residuals(object = cfit, type = "score")
    if(cfunc == "survreg"){
      rr <- residuals(object = cfit, type = "matrix")
      dldg <- rr[, "dg"]
      dgdx <- model.matrix(object = cfit)
      cres <- dldg*dgdx
      if(nrow(cfit$var) > length(cfit$coef)) cres <- cbind(cres, rr[, "ds"])
    }
    dldg <- residuals(object = efit, type = "response")
    dgdx <- model.matrix(object = efit)
    eres <- dldg*dgdx

    cvar <- -solve(cfit$var)/N
    evar <- -solve(vcov(object = efit))/N
  }
}

#---LOOP OVER TIMES---

for(k in 1:length(times)){

  t <- times[k]
```

```
if(method == "ML"){
  S <- ML.fun()
  Stres <- S[, 1]
  St0res <- S[, 2]
  if(se.fit){
    res <- cbind(Stres, St0res, ores)
    #this subsetting is needed because cov.wt does not have a na.rm argument
    complete <- complete.cases(res)
    res <- res[complete, ]
    wt <-  weights[complete]
    #weighted covariance is needed because res is created with the residual
    #function, which gives unweighted residuals
    J <- cov.wt(x = res, wt = wt)$cov
    if(ofunc == "survreg")
      theta <- c(ofit$coefficients, log(ofit$scale))
    if(ofunc == "coxph")
      theta <- ofit$coefficients
    SI <- cbind(c(-1, 0), c(0, -1),
        jacobian(func = ML.fun, x = theta, method = jacobian.method))
    oI <- cbind(rep(0, nopar), rep(0, nopar), ovar)
    I <- rbind(SI, oI)
  }
}

if(method == "IPW"){
  S <- IPW.fun()
  Stres <- S[, 1]
  St0res <- S[, 2]
  if(se.fit){
    res <- cbind(Stres, St0res, cres, eres)
    #this subsetting is needed because cov.wt does not have a na.rm argument
    complete <- complete.cases(res)
    res <- res[complete, ]
    wt <-  weights[complete]
    #weighted covariance is needed because res is created with the residual
    #function, which gives unweighted residuals
    J <- cov.wt(x = res, wt = wt)$cov
    if(cfunc == "survreg")
      theta <- c(cfit$coefficients, log(cfit$scale), efit$coefficients)
    if(cfunc == "coxph")
      theta <- c(cfit$coefficients, efit$coefficients)
    SI <- cbind(c(-1, 0), c(0, -1),
        jacobian(func = IPW.fun, x = theta, method = jacobian.method))
    cI <- cbind(rep(0, ncpar), rep(0, ncpar), cvar,
        matrix(rep(0, ncpar*nepar), nrow = ncpar, ncol = nepar))
    eI <- cbind(rep(0, nepar), rep(0, nepar),
        matrix(rep(0, nepar*ncpar), nrow = nepar, ncol = ncpar), evar)
    I <- rbind(SI, cI, eI)
  }
}

if(method == "DR"){
  S <- DR.fun()
```

```
    St1res <- S[, 1]
    St0res <- S[, 2]
    if(se.fit){
      res <- cbind(St1res, St0res, ores, cres, eres)
      #this subsetting is needed because cov.wt does not have a na.rm argument
      complete <- complete.cases(res)
      res <- res[complete, ]
      wt <-  weights[complete]
      #weighted covariance is needed because res is created with the residual
      #function, which gives unweighted residuals
      J <- cov.wt(x = res, wt = wt)$cov
      theta <- NULL
      if(ofunc == "survreg")
        theta <- c(theta, ofit$coefficients, log(ofit$scale))
      if(ofunc == "coxph")
        theta <- c(theta, ofit$coefficients)
      if(cfunc == "survreg")
        theta <- c(theta, cfit$coefficients, log(cfit$scale))
      if(cfunc == "coxph")
        theta <- c(theta, cfit$coefficients)
      theta <- c(theta, efit$coefficients)
      SI <- cbind(c(-1, 0), c(0, -1),
          jacobian(func = DR.fun, x = theta, method = jacobian.method))
      oI <- cbind(rep(0, nopar), rep(0, nopar), ovar,
          matrix(rep(0, nopar*ncpar), nrow = nopar, ncol = ncpar),
          matrix(rep(0, nopar*nepar), nrow = nopar, ncol = nepar))
      cI <- cbind(rep(0, ncpar), rep(0, ncpar),
          matrix(rep(0, ncpar*nopar), nrow = ncpar, ncol = nopar), cvar,
          matrix(rep(0, ncpar*nepar), nrow = ncpar, ncol = nepar))
      eI <- cbind(rep(0, nepar), rep(0, nepar),
          matrix(rep(0, nepar*nopar), nrow = nepar, ncol = nopar),
          matrix(rep(0, nepar*ncpar), nrow = nepar, ncol = ncpar), evar)
      I <- rbind(SI, oI, cI, eI)
    }
  }

  #---ESTIMATES---

  St1 <- weighted.mean(x = St1res, w = weights, na.rm = TRUE)
  St0 <- weighted.mean(x = St0res, w = weights, na.rm = TRUE)
  est[((k-1)*3+1):((k-1)*3+3)] <- c(St1, St0, St1 - St0)

  #---STANDARD ERRORS---
  if(se.fit){
    V <- (solve(I)%*%J%*%t(solve(I))/N)[1:2, 1:2]
    #dAF.dSt.dSt0 <- matrix(c(-(1-St0)/(1-St)^2, 1/(1-St)), nrow = 2, ncol = 1)
    se[((k-1)*3+1):((k-1)*3+3)] <- c(sqrt(V[1,1]), sqrt(V[2,2]),
      sqrt(V[1,1] + V[2,2] - 2 * V[1,2]))
  }
}

if(se.fit) return(list(est = est, se = se))
else return(list(est = est))
```

```
}


set.seed(20230804)

df <- rotterdam

df$time <- pmin(df$rtime, df$dtime) / 365.25
df$status <- ifelse(df$recur == 1 | df$death == 1, 1, 0)

## exposure is chemotherapy

plot(survfit(Surv(time, status) ~ chemo, data = df), col = 1:2)

## estimate survival difference at 2.5, 5, and 7.5 years

## propensity score fit

wmod <- glm(chemo ~ year + age + meno + size +
              factor(grade) + nodes + pgr + er + hormon,
            data = df, family = binomial)

phatr <- predict(wmod, type = "response")
df$Wprop <- df$chemo / phatr + (1 - df$chemo) / (1 - phatr)

coxmod <- coxph(Surv(time, status) ~ chemo + year + age + meno +
                  size + factor(grade) + nodes + pgr + er + hormon, data = df,
      weights = Wprop, robust = TRUE, ties = "breslow")

cox.zph(coxmod)

coxmod$weights <- rep(1, coxmod$n)
stdfit <- summary(stdCoxph(coxmod, data = df, X = "chemo", t = c(2.5, 5, 7.5)),
        contrast = "difference", reference = 0)

stdres <- as.data.frame(do.call(rbind, lapply(stdfit$est.table, \(cf) cf[2, ])))
stdres$time <- c(2.5, 5, 7.5)

## bootstrap for variance

fit_std_cox <- function(df) {

  wmod <- glm(chemo ~ year + age + meno + size +
                factor(grade) + nodes + pgr + er + hormon,
              data = df, family = binomial)

  phatr <- predict(wmod, type = "response")
  df$Wprop <- df$chemo / phatr + (1 - df$chemo) / (1 - phatr)

  coxmod <- coxph(Surv(time, status) ~ chemo + year + age + meno +
                    size + factor(grade) + nodes + pgr + er + hormon, data = df,
                  weights = Wprop, robust = TRUE, ties = "breslow")
```

```
  coxmod$weights <- rep(1, coxmod$n)
  stdfit <- summary(stdCoxph(coxmod, data = df, X = "chemo",
                             t = c(2.5, 5, 7.5)),
                    contrast = "difference", reference = 0)

  stdres <- as.data.frame(do.call(rbind,
        lapply(stdfit$est.table, \(cf) cf[2, ])))
  stdres$Estimate

}


bootcoxstd <- lapply(1:1000, \(i) {
  dfstar <- df[sample(1:nrow(df), nrow(df), replace = TRUE),]
  fit_std_cox(dfstar)
})

bootcoxstdmat <- do.call(rbind, bootcoxstd)
stdres$`Std. Error Boot` <- apply(bootcoxstdmat, 2, sd)

df$censor <- 1 - df$status
drFit <-
  afSurvival(
    oformula = Surv(time, status) ~ chemo + year + age + meno +
      size + factor(grade) + nodes + pgr + er + hormon,
    ofunc = "survreg",
    cformula = Surv(time, censor) ~ chemo + year + age,
    cfunc = "survreg",
    eformula = chemo ~ year + age + meno + size +
      factor(grade) + nodes + pgr + er + hormon,
    method = "DR",
    times = c(2.5, 5, 7.5),
    se.type = "sandwich",
    data = df
  )


drFitboot <-
  afSurvival(
    oformula = Surv(time, status) ~ chemo + year + age + meno +
      size + factor(grade) + nodes + pgr + er + hormon,
    ofunc = "survreg",
    cformula = Surv(time, censor) ~ chemo + year + age,
    cfunc = "survreg",
    eformula = chemo ~ year + age + meno + size +
      factor(grade) + nodes + pgr + er + hormon,
    method = "DR",
    times = c(2.5, 5, 7.5),
    se.type = "boot",
    data = df
  )
```

```
dfF <- df
dfF$chemo <- factor(dfF$chemo)
binfits <-
  rbind(
    summary(
      logitIPCWATE(
        Event(time, status) ~ chemo + year + age + meno +
          size + factor(grade) + nodes + pgr + er + hormon,
        data = dfF,
        time = 2.5,
        treat.model = chemo ~ year + age +
          meno + size + factor(grade) + nodes + pgr + er + hormon
      )
    )$ateDR[3,],
    summary(
      logitIPCWATE(
        Event(time, status) ~ chemo + year + age + meno +
          size + factor(grade) + nodes + pgr + er + hormon,
        data = dfF,
        time = 5,
        treat.model = chemo ~ year + age +
          meno + size + factor(grade) + nodes + pgr + er + hormon
      )
    )$ateDR[3,],
    summary(
      logitIPCWATE(
        Event(time, status) ~ chemo + year + age + meno +
          size + factor(grade) + nodes + pgr + er + hormon,
        data = dfF,
        time = 7.5,
        treat.model = chemo ~ year + age +
          meno + size + factor(grade) + nodes + pgr + er + hormon
      )
    )$ateDR[3,]
  )

binfits <- as.data.frame(binfits)
binfits[, c(1, 3, 4)] <- -binfits[, c(1, 3, 4)]
binfits$time <- c(2.5, 5, 7.5)
colnames(binfits)[3:4] <- c("upperCI", "lowerCI")


## pseudo



## pseudo observations -- bootstrap for variance
fit_pseudo <- function(df, tt) {
  wmod <-
    glm(
      chemo ~ year + age + meno + size + factor(grade) +
        nodes + pgr + er + hormon,
      data = df,
      family = binomial
```

```
    )

  phatr <- predict(wmod, type = "response")
  df$Wprop <- df$chemo / phatr + (1 - df$chemo) / (1 - phatr)

  ofitr <-
    cumincglm(
      Surv(time, status) ~ chemo + year + age + meno +
        size + factor(grade) + nodes + pgr + er + hormon,
      data = df,
      time = tt,
      link = "cloglog"
    )

  df1 <- df0 <- df
  df1$chemo <- 1
  df0$chemo <- 0

  dr1rw <-
    ofitr$y * (df$chemo == 1) / phatr -
    predict(ofitr, newdata = df1, type = "response") *
    ((df$chemo == 1) - phatr) / phatr
  dr0rw <-
    ofitr$y * (df$chemo == 0) / (1 - phatr) +
    predict(ofitr, newdata = df0, type = "response") *
    ((df$chemo == 1) - phatr) / (1 - phatr)


  sdiffs.po <- -1 * c(mean(dr1rw) - mean(dr0rw))
  sdiffs.po
}

mainps <- c(fit_pseudo(df, 2.5),
            fit_pseudo(df, 5),
            fit_pseudo(df, 7.5))

bootps <- lapply(1:1000, \(i) {
  dfb <- df[sample(1:nrow(df), nrow(df), replace = TRUE),]
  c(fit_pseudo(dfb, 2.5),
    fit_pseudo(dfb, 5),
    fit_pseudo(dfb, 7.5))
})

bootps <- do.call(rbind, bootps)
se.ps <- apply(bootps, 2, sd)


sdiffs.po <- as.data.frame(cbind(mainps, se.ps))
sdiffs.po$time <- c(2.5, 5, 7.5)
sdiffs.po$model <- "pseudo"

## summary table
```

```
stab <- rbind(
  data.frame(
    est = stdres$Estimate,
    se = stdres$`Std. Error`,
    time = c(2.5, 5, 7.5),
    model = "standardized IPTW Cox"
  ),
  data.frame(
    est = stdres$Estimate,
    se = stdres$`Std. Error Boot`,
    time = c(2.5, 5, 7.5),
    model = "standardized IPTW Cox"
  ),
  data.frame(
    est = drFit$est.AF,
    se = drFit$se.AF,
    time = c(2.5, 5, 7.5),
    model = "DR survival"
  ),
  data.frame(
    est = drFit$est.AF,
    se = drFitboot$se.AF,
    time = c(2.5, 5, 7.5),
    model = "DR survival"
  ),
  data.frame(
    est = binfits$Estimate,
    se = binfits$Std.Err,
    time = c(2.5, 5, 7.5),
    model = "DR binomial regression"
  ),
  data.frame(
    est = sdiffs.po$mainps,
    se = sdiffs.po$se.ps,
    time = c(2.5, 5, 7.5),
    model = "DR pseudo observations"
  )
)

stab$lower95 <- with(stab, est - 1.96 * se)
stab$upper95 <- with(stab, est + 1.96 * se)

library(xtable)
print(xtable(stab[order(stab$time),c(4, 1, 2, 5, 6)],
             digits = 3), include.rownames = FALSE)
```

# References


Per K Andersen, Ornulf Borgan, Richard D Gill, and Niels Keiding. *Statistical models based on counting processes*. Springer Science & Business Media, 2012.

Paul Frederic Blanche, Anders Holt, and Thomas Scheike. On logistic regression with right censored data,

with or without competing risks, and its use for estimating treatment effects. *Lifetime data analysis*, 29 (2):441–482, 2023.

AG DiRienzo and SW Lagakos. Effects of model misspecification on tests of no randomized treatment effect arising from cox's proportional hazards model. *Journal of the Royal Statistical Society: Series B (Statistical Methodology)*, 63(4):745–757, 2001.

Fan Hui Kong and Eric Slud. Robust covariate-adjusted logrank tests. *Biometrika*, 84(4):847–862, 1997.

D. Y. Lin and L. J. Wei. The robust inference for the cox proportional hazards model. *Journal of the American Statistical Association*, 84(408):1074–1078, 1989.

Michael C. Sachs and Erin E. Gabriel. Event history regression with pseudo-observations: Computational approaches and an implementation in R. *Journal of Statistical Software*, 102(9):1–34, 2022. doi: 10.18637/jss.v102.i09.

Arvid Sjölander and Stijn Vansteelandt. Doubly robust estimation of attributable fractions in survival analysis. *Statistical methods in medical research*, 26(2):948–969, 2017.

C. A. Struthers and J. D. Kalbfleisch. Misspecified proportional hazard models. *Biometrika*, 73(2):363–369, 1986. ISSN 00063444. URL `http://www.jstor.org/stable/2336212`.

Jixian Wang. A simple, doubly robust, efficient estimator for survival functions using pseudo observations. *Pharmaceutical Statistics*, 17(1):38–48, 2018. doi: https://doi.org/10.1002/pst.1834. URL `https://onlinelibrary.wiley.com/doi/abs/10.1002/pst.1834`.
